# Supplementary material for: Modelling the efficacy of hyperthermia treatment
Source: arXiv:1209.3924 source file (2013-03-06)
Supplement: Supplementary file 1 [file file_si-termotolerancja.pdf]

# Modelling the efficacy of hyperthermia treatment

Mikołaj Rybiński[1,2], Zuzanna Szymańska[3], Sławomir Lasota[1] and Anna Gambin[1,2]

[1] Institute of Informatics, University of Warsaw, Poland
[2] Mossakowski Medical Research Centre, Polish Academy of Sciences, Poland
[3] Interdisciplinary Centre for Mathematical and Computational Modelling, University of Warsaw, Poland

This is supplementary material for the paper *Modelling the efficacy of hyperthermia treatment.*

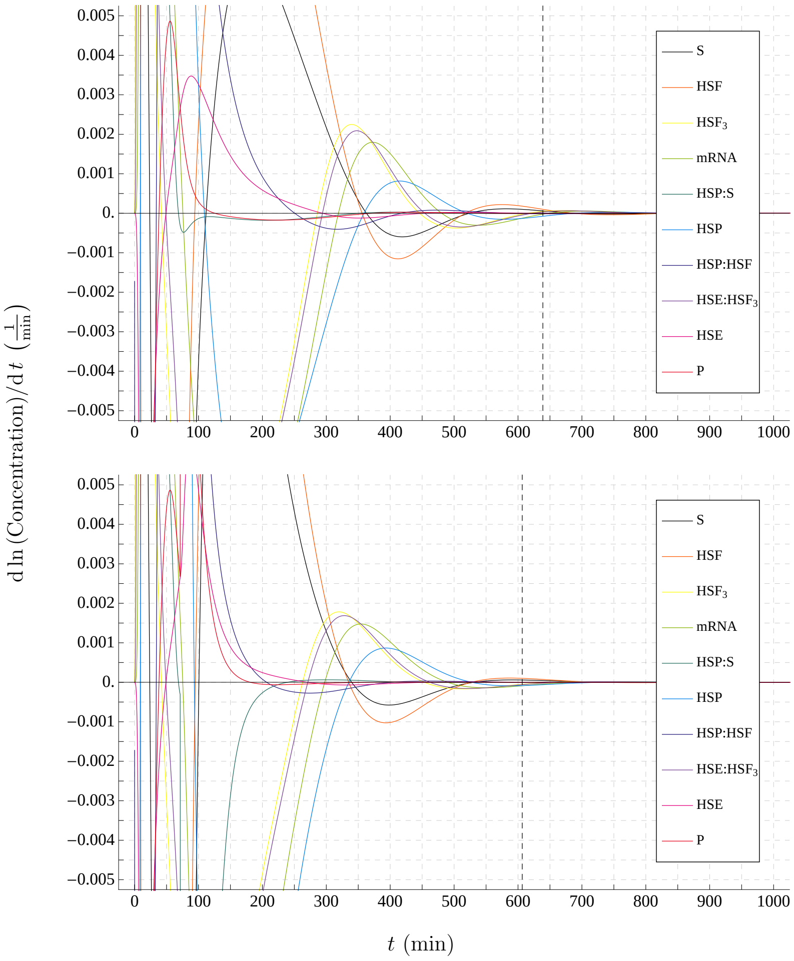


**Fig. S1:** Stability of the HSR ODE model for immediate T $= 42^{\circ}$C: constitutive heat-shock (upper plot); heat-shock ended after 71 $\mathrm{min}$ (lower plot). Normalised change rate of all species is plotted against time. Normalised change rate is represented as a log-concentration derivative, which is approximated by a $\Delta t = 0.1\ \mathrm{min}$ differential for ODE numerical solutions, i.e., $\frac{\mathrm{d}\ln(x(t))}{\mathrm{d}\,t} \approx \frac{x(t+\Delta t)-x(t)}{\Delta t} \cdot \frac{1}{x(t)}$, where $x$ is an ODE variable representing species concentration. We assume that system completely stabilises when normalised change rate of all species goes and stays under $10^{-4}\ \frac{1}{\mathrm{min}}$, i.e., at ca. 639 $\mathrm{min}$ for the constitutive heat-shock (vertical black dashed line in the upper plot) and at ca. 607 $\mathrm{min}$ for the heat-shock ended at 71 $\mathrm{min}$ (vertical black dashed line in the lower plot).

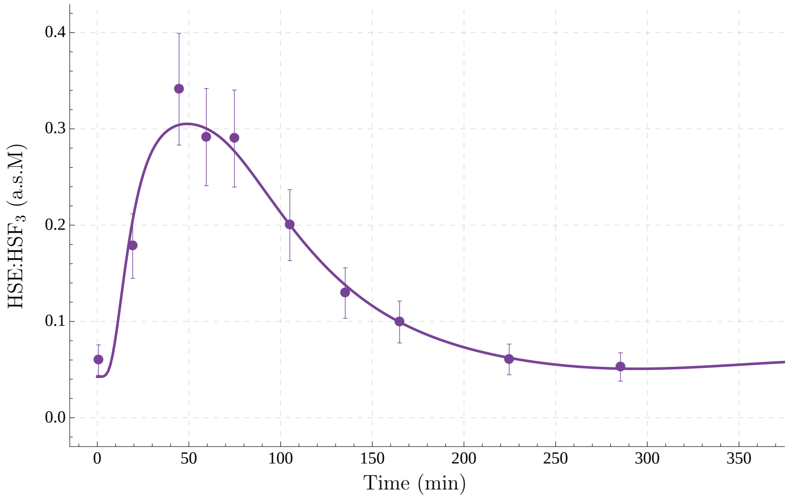


**Fig. S2:** The HSE:HSF$_3$ fit to the experimental data ([1], Fig. 8A), for a constitutive 42°C heat-shock. We assumed relative 15% error plus 2% of the peak value. The resulting fit gives $\chi^2\,(10)$=2.49 (with p-value equal to 99%), for concentration scale equal to $7.3\times10^{-3}$ "levels" to arbitrary scale molars $(\mathrm{a.s.M})$.

**Text S3: Stochastic modelling of HSR** In this supplementary text we give a detailed description and comparison of our HSR deterministic and stochastic mathematical models. This text also contains detailed description of how exactly we applied PMC in this work and how we implemented the stochastic perturbation strategy.Text is avaialable at the end of this document.

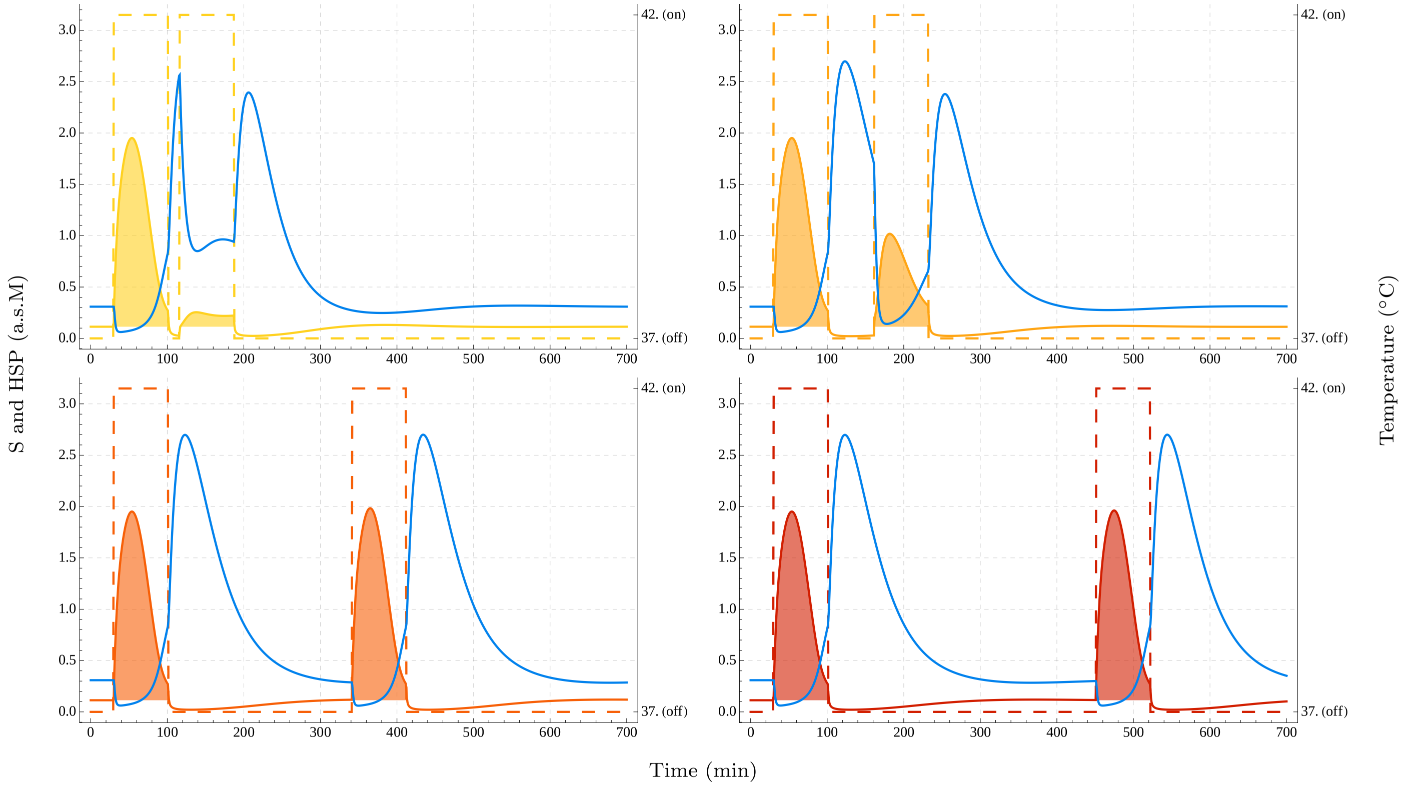


**Figure S4:** The substrate (coloured area) and HSP (blue line) response to the two consecutive immediate heat-shocks. Duration and strength of the memory of the first temperature perturbation can be tracked by the activity of the free HSP. Its level at the moment when the second heat-shock is induced is negatively correlated with the strength of the second response. Shortly after the first heat-shock, a HSP level is still high. At that moment there are chaperon proteins ready to act immediately. When a second heat-shock is applied (upper left) there is no delay caused by the need of synthesis of new HSP proteins, as was in a case of the first heat-shock. Thus, no significant amount of the toxic substrate is observed. With time amount of HSP returns to the stable homeostasis level, going through medicore HSP and the substrate response (upper right). At the time point of HSP stabilisation the memory of the first heat-shock is completely lost (lower right). However, shortly before that happens, amount of HSP is slightly smaller than at the homeostasis. When a second heat-shock is applied at such time point (lower left), the amount of newly synthesised HSP required for the response is larger. Thus, the response is slower than in the first instance of stress conditions. In effect, substrate has more time to reach an even higher level than previously.

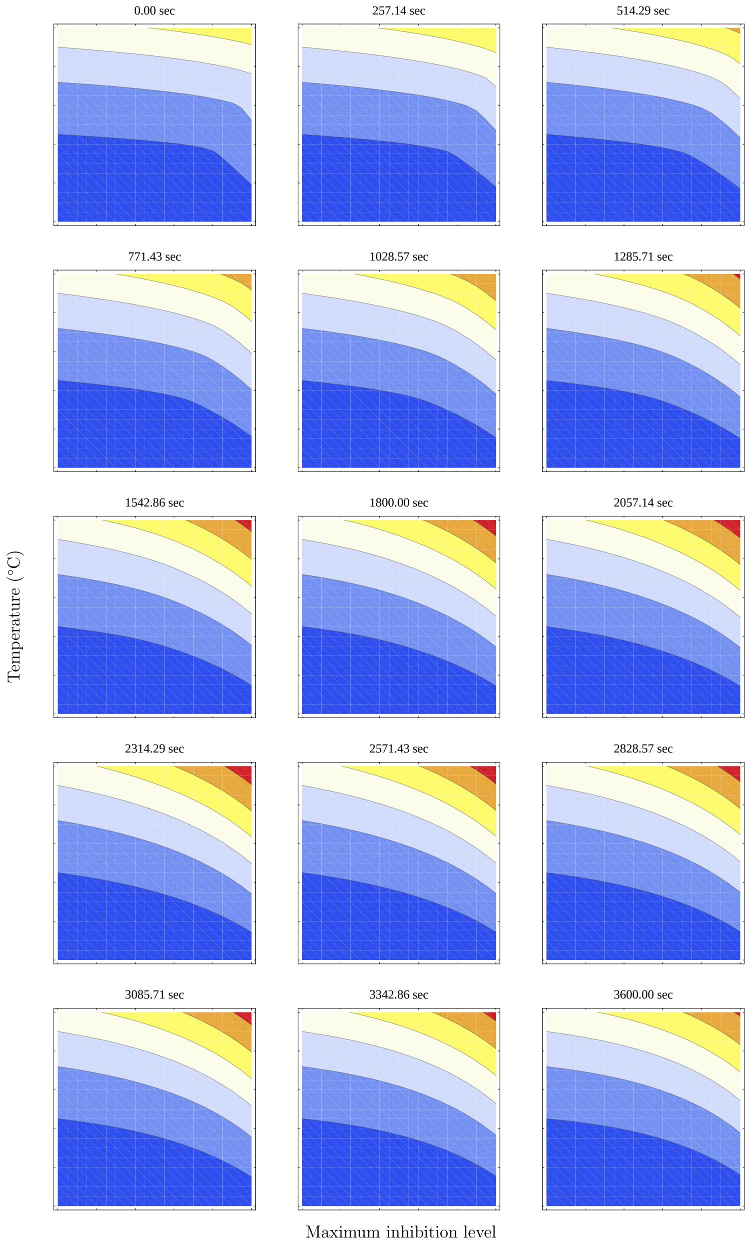


**Figure S5:** Contour plots of the heat-shock response level $\mathcal{R}_1$ with respect to a heat-shock temperature (vertical axes) and with respect to a maximum level of proteasome inhibition (horizontal axes) for multiple equally-distributed heat-shock application times $t_1$ in range 0–60 $\mathrm{min}$. Vertical axes have linear scale of 37–42°C; horizontal axes have linear scale of 0–100%; $\mathcal{R}_1$ values are categorised into $[0, 0.5), \ldots [3, 3.5)$ intervals, represented by discrete colour spectrum going from blue to red.

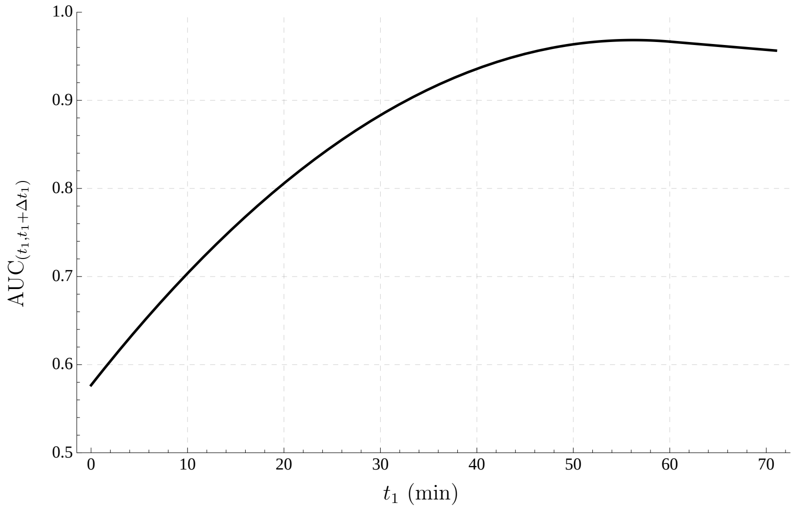


**Figure S6:** Area under the bortezomib inhibition curve (AUC) versus heat-shock application time $t_1$, for a fixed heat-shock duration $\Delta t_1 = 71$ min. More specifically, $\mathrm{AUC}_{(t_1,t_1+\Delta t_1)} = \int_{t_1}^{t_1+\Delta t_1} \mathrm{I}(t)/\mathrm{I}_{100}\,\mathrm{d}\,t$; maximum value is reached for $t_1 = 56.24$ min.

# Text S3: Stochastic modelling of HSR

## S3.1: Model

Table 1 gives reaction list with kinetic parameters, whereas Table 2 gives the implied mass conservation constraints. Structural changes with respect to the previous version of this model by Szymańska and Żylicz [8] include explicit native protein species (Eqs (r9) and (r10)) and separate HSP mRNA degradation (Eqs (r11) and (r12)).

$$\mathrm{HSP{:}HSF} + \mathrm{S} \underset{\mathrm{l}_6}{\overset{\mathrm{k}_6}{\rightleftharpoons}} \mathrm{HSP{:}S} + \mathrm{HSF}, \tag{r1}$$

$$3 \cdot \mathrm{HSF} \xrightarrow{\mathrm{k}_3} \mathrm{HSF}_3, \tag{r2}$$

$$\mathrm{HSF}_3 + \mathrm{HSE} \underset{\mathrm{l}_7}{\overset{\mathrm{k}_7}{\rightleftharpoons}} \mathrm{HSE{:}HSF}_3, \tag{r3}$$

$$\mathrm{HSE{:}HSF}_3 \xrightarrow{\mathrm{k}_8} \mathrm{HSE{:}HSF}_3 + \mathrm{mRNA}, \tag{r4}$$

$$\mathrm{HSP} + \mathrm{HSF}_3 \xrightarrow{\mathrm{l}_3} \mathrm{HSP{:}HSF} + 2 \cdot \mathrm{HSF}, \tag{r5}$$

$$\mathrm{HSP} + \mathrm{S} \underset{\mathrm{l}_1}{\overset{\mathrm{k}_1}{\rightleftharpoons}} \mathrm{HSP{:}S}, \tag{r6}$$

$$\mathrm{HSP} + \mathrm{HSF} \underset{\mathrm{l}_2}{\overset{\mathrm{k}_2}{\rightleftharpoons}} \mathrm{HSP{:}HSF}, \tag{r7}$$

$$\mathrm{HSP} \xrightarrow{\mathrm{k}_9} \emptyset, \tag{r8}$$

$$\mathrm{HSP{:}S} \xrightarrow{\mathrm{k}_{10}} \mathrm{HSP} + \mathrm{P}, \tag{r9}$$

$$\mathrm{P} \xrightarrow{\mathrm{k}_{11}^{\mathrm{T}}} \mathrm{S}, \tag{r10}$$

$$\mathrm{mRNA} \xrightarrow{\mathrm{k}_4} \mathrm{mRNA} + \mathrm{HSP}, \tag{r11}$$

$$\mathrm{mRNA} \xrightarrow{\mathrm{k}_5} \emptyset. \tag{r12}$$

**Table 1:** The HSR biochemical reactions network. There are 12 reactions (r1)–(r12), 4 of which are reversible, making it 16 reactions in total; $\mathrm{l}_i$ $(i = 1, 2, 6, 7)$ denotes reverse reaction rate constant. The T superscript denotes a temperature dependence.

Tables 3 and 4 summarise, respectively, the variables of the model with their initial values, as well as description and values of all kinetic parameters. Parameters $\mathrm{k}_i$, and $\mathrm{l}_j$ denote the mass action reaction rates constants, respectively, for the forward and backward reactions. Value of the reaction rate constant $\mathrm{k}_{11}^{\mathrm{T}}$ depends on the given temperature T; more

$$\begin{aligned}
\mathrm{P_{tot}} &= \mathrm{P}(t) + \mathrm{S_{tot}}(t), \\
&\quad \text{where } \mathrm{S_{tot}}(t) = \mathrm{S}(t) + \mathrm{HSP{:}S}(t), && \text{(c1)} \\
\mathrm{HSF_{tot}} &= \mathrm{HSF}(t) + \mathrm{HSP{:}HSF}(t) + 3 \cdot \mathrm{HSF_3}(t) + \\
&\quad + 3 \cdot \mathrm{HSE{:}HSF_3}(t), && \text{(c2)} \\
\mathrm{HSE_{tot}} &= \mathrm{HSE{:}HSF_3}(t) + \mathrm{HSE}(t). && \text{(c3)}
\end{aligned}$$

**Table 2:** Mass conservation laws in the HSR biochemical reactions network. Neither concentrations nor molecules numbers are annotated because Eqs (c1)–(c3) hold for all $t \geq 0$ in both deterministic and stochastic models.

specifically:

$$\mathrm{k}_{11}^{\mathrm{T}} \approx \mathrm{m}_{11} \times \left(1 - \frac{0.4}{\exp^{\Delta \mathrm{T}}}\right) \times 1.4^{\Delta \mathrm{T}} \quad \mathrm{min}^{-1}, \tag{1}$$

where $\Delta\mathrm{T} = \mathrm{T} - 37$ is a heat-shock temperature delta and $\mathrm{m}_{11} = 0.0105$ is a time-scale dependent multiplier. This function was originally proposed by Peper et al. [6], and recently reused in several other works [8, 7, 5]. Eq. (1) is valid in a local temperature range, i.e., for $\mathrm{T} \in [37, 45]\,^\circ\mathrm{C}$ [6]. We had to adjust $\mathrm{m}_{11}$ to the time scale (min) and to the original experimental data of Lepock et al. [3] (cf. [7, 5]).

| | **Description** | **Value** |
|---|---|---|
| HSP | free HSP | 0.309 |
| HSF | HSF monomers | 0.151 |
| S | substrate (denatured/misfolded protein) | 0.113 |
| HSP:HSF | HSP:HSF interacting complexes | 2.588 |
| HSP:S | HSP:substrate complexes | 1.126 |
| $\mathrm{HSF_3}$ | active HSF (trimer form) | 0.044 |
| HSE | free HSE | 0.957 |
| $\mathrm{HSE{:}HSF_3}$ | bound HSE | 0.043 |
| mRNA | HSP mRNA | 0.115 |
| P | native proteins (denaturation susceptible) | 8.761 |

**Table 3:** Description of variables used in the HSR model, together with initial conditions for the deterministic version. These are a steady state concentrations in a non stressed cells ($\mathrm{T} = 37^\circ\mathrm{C}$; see text for detail). Values are given in *arbitrary scale* molar concentration (a.s.M).

| | Rate constant of... | Value |
|---|---|---|
| $k_1$ | HSP:substrate association | 1.47 |
| $l_1$ | HSP:substrate dissociation | 0.0175 |
| $k_2$ | HSP:HSF association | 1.47 |
| $l_2$ | HSP:HSF dissociation | 0.0175 |
| $k_3$ | HSF trimers association (activation) | 0.0805 |
| $l_3$ | HSF trimers dissociation (inactivation) | 0.020125 |
| $k_4$ | HSP translation | 0.1225 |
| $k_5$ | HSP mRNA degradation | 0.0455 |
| $k_6$ | HSP:HSF dissociation and HSP:substrate association | 0.0805 |
| $l_6$ | HSP:substrate dissociation and HSP:HSF association | 0.00126 |
| $k_7$ | HSE:$HSF_3$ association | 0.1225 |
| $l_7$ | HSE:$HSF_3$ dissociation | 0.1225 |
| $k_8$ | HSP mRNA transcription | 0.1225 |
| $k_9$ | HSP degradation | 0.0455 |
| $k_{10}$ | misfolded protein refolding (substrate degradation) | 0.049 |
| $k_{11}^{T}$ | protein misfolding (substrate production) | Eq. (1) |

**Table 4:** HSR model parameters. All values, except for $k_5$ are taken directly from the Szymańska and Żylicz [8] model and scaled for the experimental data fit. Note that all mass action rate constants (i.e. $k_i$ and $l_j$) have units $\min^{-1}(\text{a.s.M})^{-\operatorname{rank}(R)+1}$, where $\operatorname{rank}(R)$ is a rank of reaction $R$, i.e., a sum of left-hand side stoichiometric coefficients.

**Deterministic framework.** As mentioned, all reaction channels follow the mass action kinetics. The $i^{\text{th}}$ substrate amount in the rate of $j^{\text{th}}$ reaction is raised to the power of its' stoichiometric coefficient $n_{ij}$, where $N = (n_{ij}) \in \mathbb{N}^{10} \times \mathbb{N}^{16}$ denotes stoichiometry matrix of total of ten species involved in sixteen reactions, as described by Eqs (r1)–(r12).

In context of the deterministic modelling framework, state of our system is represented by the time dependent state vector $\mathbf{y}(t)$ of concentrations of reacting species $y_i$ $(i = 1 \dots 10)$. Given the initial state $\mathbf{y}_0$ (see Table 3), the dynamics of the system is governed by a set of 10 *ordinary differential equations* (ODE), called *reaction rate equations* (RRE):

$$\frac{\mathrm{d}\,\mathbf{y}(t)}{dt} = \mathbf{f}(\mathbf{y}(t)) = N\mathbf{v}(\mathbf{y}(t)), \tag{2}$$

where $\mathbf{v}(\mathbf{y}(t)) \in \mathbb{R}^{16}$ is a vector of reaction rates at a time point $t$.

**Stochastic extension.** In the stochastic approach we provide a set of linear, autonomous ODE, one for each possible state of the system. Such set of equations is called the *chemical master equation* (CME). The solution of the $k$-th equation at a time point $t$ corresponds to the probability of the system being in that particular state at that time $t$. The system

state is encoded as a vector $\mathbf{X}(t) \in \mathbb{N}^{10}$ containing molecule numbers of all species. The $j$-th reaction changes the molecule numbers by:

$$\mathbf{X}(t) \to \mathbf{X}(t) + \mathbf{n}_j,$$

where $\mathbf{n}_j$ is the $j$-th column of $N$. Denote by $a_j(\mathbf{X}(t))$ the propensity function associated with the $j$-th reaction. Probability of $j$-th reaction taking place in the infinitesimally small time interval $[t, t+dt)$ is accurately approximated by $a_j(\mathbf{X}(t))dt$. CME describing the time-dependent distribution $P(\mathbf{x}, t)$ of system states, i.e. the probability that $\mathbf{X}(t) = \mathbf{x}$, is given by:

$$\frac{\mathrm{d}\, P(\mathbf{x}, t)}{dt} = \sum_j a_j(\mathbf{x} - \mathbf{n}_j) P(\mathbf{x} - \mathbf{n}_j, t) - \sum_j a_j(\mathbf{x}) P(\mathbf{x}, t). \qquad (3)$$

Because the propensity functions $a_j$ are time-independent, the CME represents a *continuous-time Markov process* (CTMC). More precisely, the solution of the CME gives the transient probabilities for all states of the CTMC.

For a stochastic model we used the scaling coefficient $\delta$ which relates concentrations in the deterministic model to the number of molecules in the stochastic model. Value of $\delta$ corresponds to a number of molecules per one unit of concentration, i.e. $\delta \cdot [S] = \#S$. This approach is equivalent to considering approximate stochastic model of packs of $N_{\mathrm{A}} \cdot |V|/\delta$ molecules instead of single molecules (here $N_{\mathrm{A}}$ is Avogadro constant and $|V|$ is the solution volume). Given HeLa cell volume of circa 2500 $\mu\mathrm{m}^3 = 2.5 \cdot 10^{-12}$ $\mathrm{dm}^3$ [4], we have that for $\delta \approx 1.5 \cdot 10^{12}$ the stochastic model is accurate. We adjust reactions constants accordingly, with $N_{\mathrm{A}} \cdot |V| := \delta$ (cf. [2]).

**Mean comparison.** We find that for $\delta = 100$ the RRE model is in a good agreement with the stochastic variant for both 37°C and 42°C. Visual comparison of ODE and stochastic simulations is presented in Figure 1. Table 5 presents comparison of stochastic mean value with RRE values for $\delta$ equal to 100 and 1000. Sources of stochastic model error are two-fold: the rounding errors due to the molecules packaging and the propensity constants approximations, especially for the only reaction with $\operatorname{rank}(R) > 1$, i.e. the HSF trimerisation (Eq. r2). Although for $\delta = 1000$ the relative error in steady state is ca. 10 times lower, the stochastic simulation paths, and, consequently, their running time, are almost exactly 10 times longer (mean 677092.4 +/− 1235.8 SD steps of

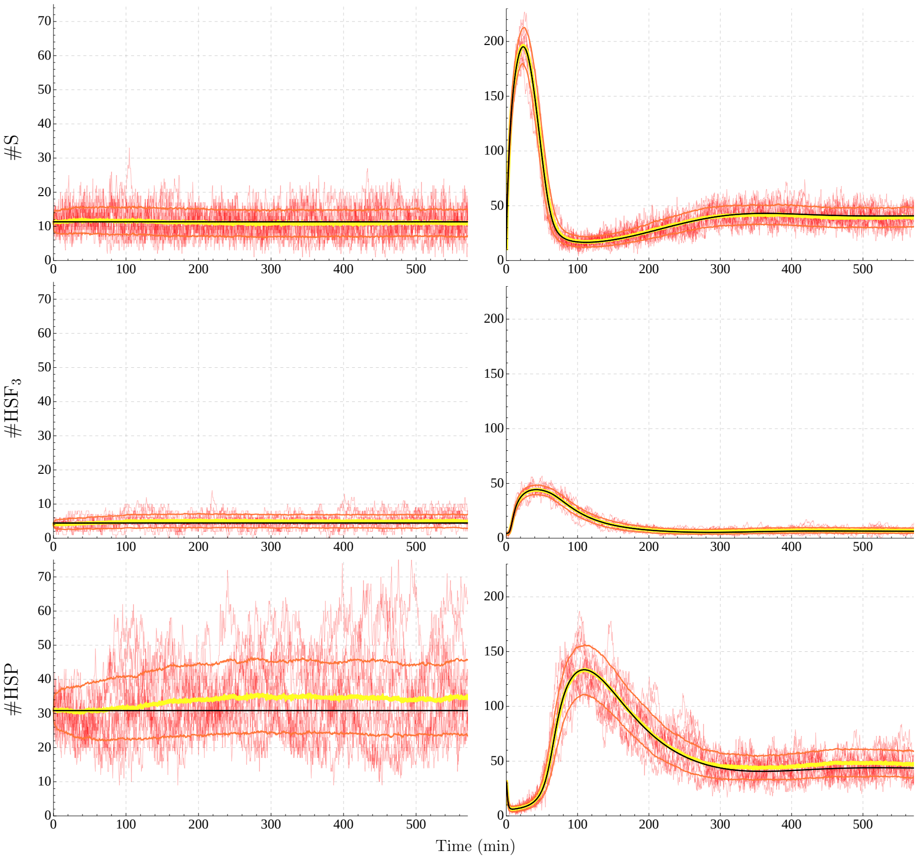


**Figure 1:** Comparison of the stochastic simulations with respect to ODE' numerical solutions for the HSR model. Both homeostasis (left column) and heat-shock (right column) conditions are compared. Each plots shows 10 sample stochastic trajectories, estimated mean $+/-$ standard deviation of a sample of $10^3$ stochastic simulations, and an ODE numerical solution (black). Here, we assumed 100 molecules per unit of concentration, i.e. $\delta = 100$.

the underlying CTMC for $\delta = 1000$ vs. mean $67722.5 +/- 396.1$ SD steps for $\delta = 100$ to reach 571 min; estimated from 1000 simulations). We find $\delta = 100$ to be a good compromise between accuracy and efficiency for our proof-of-concept case study.

**Level of stochastic noise.** The *variance-to-mean ratio*:

$$\mathrm{VMR}\,(X) = \frac{\mathrm{Var}\,(X)}{\mathbb{E}\,(X)}$$

Relative error +/− 95% confidence interval in %

| Species | Homeostasis | | Heat-shock | |
|---|---|---|---|---|
| | $\delta$=100 | $\delta$=1000 | $\delta$=100 | $\delta$=1000 |
| HSP | 12.5 +/− .68 | 1.31 +/− .19 | 8.4 +/− .55 | 0.83 +/− .16 |
| $HSF_3$ | 12.1 +/− .86 | 1.45 +/− .26 | 9.4 +/− .75 | 0.71 +/− .23 |
| HSP mRNA | 12.1 +/− .79 | 1.23 +/− .24 | 8.8 +/− .67 | 0.79 +/− .21 |
| $HSE{:}HSF_3$ | 11.4 +/− .87 | 1.37 +/− .26 | 8.5 +/− .74 | 0.86 +/− .23 |
| HSF | 6.9 +/− .72 | 0.88 +/− .24 | 5.1 +/− .68 | 0.76 +/− .23 |
| substrate | 2.5 +/− .69 | 0.34 +/− .22 | 2.9 +/− .44 | 0.33 +/− .14 |
| HSP:HSF | 1.6 +/− .06 | 0.21 +/− .02 | 1.8 +/− .09 | 0.21 +/− .03 |
| HSE | 0.6 +/− .04 | 0.06 +/− .01 | 0.5 +/− .05 | 0.05 +/− .01 |
| HSP:substrate | 0.1 +/− .17 | 0.04 +/− .05 | 0.1 +/− .05 | 0.01 +/− .02 |

**Table 5:** Estimates of a relative error of each species mean value with respect to its RRE value, i.e. $|\mathbb{E}(\#S) - [S]|/[S]$; values are given in percent. Relative errors were calculated in homeostasis (T = 37°C) and the heat shock steady state (T = 42°C), for two scaling coefficient $\delta$ values. Species are sorted according to error values in homeostasis for $\delta = 100$; from the least to the most consistent with the RRE solutions. Steady state mean values were estimated using APMC with $10^4$ independent simulation samples for each species.

quantifies noise of a species amount variable $X = \#S$ at a fixed time point in the stochastic model, with respect to the Poisson birth-death process (see, e.g., [9]). Table 6 contains estimated steady state values of VMR in our stochastic HSR model. These VMR values are significant for some of the crucial species, both for the state of homeostasis and the steady state during the heat-shock.

The steady state amount of substrate, HSP, HSF and HSP mRNA is over-dispersed with respect to the Poisson distribution, indicating their high stochasticity in our model. In general, the relative noise of species amounts increases for the higher temperature parameter value: mean VMR is 1.23 in homeostasis, whilst it is 1.32 in the 42°C heat-shock (ca. 7.5% higher; see Table 6). This is only due to the almost two-fold increase in the substrate noise (highlighted).

### S3.2: Reward-based estimators

Steady state mean value of amount of each species was estimated using the confidence interval APMC method to verify the reward-based property:

$$\mathrm{R}_{\{\#S=?\}}\,(\mathrm{I} = \text{burn-in time})\,,$$

where $\#S$ reward for each species $S$ is defined as:

```
rewards "#S" true : S; endrewards
```

| Species | Homeostasis | Heat-shock |
|---|---|---|
| | VMR +/− 95% confidence interval | |
| HSP | 3.05 +/− 0.65 | 3.14 +/− 0.74 |
| HSF | 2.41 +/− 0.35 | 2.21 +/− 0.40 |
| HSP mRNA | 1.68 +/− 0.29 | 1.60 +/− 0.34 |
| substrate | 1.19 +/− 0.24 | 2.32 +/− 0.53 |
| HSE:$HSF_3$ | 0.81 +/− 0.12 | 0.85 +/− 0.14 |
| HSP:substrate | 0.78 +/− 0.55 | 0.57 +/− 0.77 |
| $HSF_3$ | 0.78 +/− 0.12 | 0.79 +/− 0.15 |
| HSP:HSF | 0.27 +/− 0.46 | 0.38 +/− 0.60 |
| HSE | 0.10 +/− 0.11 | 0.03 +/− 0.13 |

**Table 6:** Estimates of VMR for each species in homeostasis (T $= 37°$C) and the heat-shock steady state (T $= 42°$C). VMR estimates were calculated for $\delta$=100. Species are sorted according to the VMR values in homeostasis; from the most to the least disperse. Dashed, vertical line separates the over-dispersed and under-dispersed variables, with respect to the Poisson distribution. The dispersion doesn't change much with temperature, except for the substrate (highlighted). Mean and variance values were estimated using APMC with, respectively, $10^4$ and $5 \cdot 10^4$ independent simulation samples for each species.

We start the stochastic process with a single point distribution, according to RRE steady state values. Therefore, to reach the steady-state distribution we wait (burn-in) for 300 min for T $=$ 37°C and 600 min for T $=$ 42°C (cf. Figure 1).

It is impossible to query for higher central moments in PRISM in a single run. Therefore, the variance value of amount of each species was estimated from the unbiased mean value and second moment estimators, i.e.

$$\widehat{\mathrm{Var}\,(X)} = \widehat{\mathbb{E}\,(X^2)} - \widehat{\mathbb{E}\,(X)}^2.$$

Second moment $\widehat{\mathbb{E}\,(\#S^2)}$ of species amount was estimated analogously to the mean value, using the confidence interval APMC method (see above). Having symmetric confidence intervals:

$$\mathbb{E}\,(X) \in \left(\widehat{\mathbb{E}\,(X)} - a_1, \widehat{\mathbb{E}\,(X)} + a_1\right) \quad \text{and}$$
$$\mathbb{E}\,(X) \in \left(\widehat{\mathbb{E}\,(X^2)} - a_2, \widehat{\mathbb{E}\,(X^2)} + a_2\right),$$

with $\alpha$ confidence level, the unbiased moments-based variance estimator $\widehat{\mathrm{Var}\,(X)}$ has an asymmetric confidence interval:

$$\begin{aligned}\underline{\mathrm{Var}\,(X)} := \left(\widehat{\mathbb{E}\,(X^2)} - a_2\right) - \left(\widehat{\mathbb{E}\,(X)} + a_1\right)^2 \\ \leq \widehat{\mathrm{Var}\,(X)} \leq \\ \left(\widehat{\mathbb{E}\,(X^2)} + a_2\right) - \left(\widehat{\mathbb{E}\,(X)} - a_1\right)^2 =: \overline{\mathrm{Var}\,(X)}.\end{aligned} \tag{4}$$

Analogously, for an unbiased VMR estimator $\widehat{\mathrm{VMR}\,(X)} = \widehat{\mathrm{Var}\,(X)}\Big/\widehat{\mathbb{E}\,(X)}$, we get asymmetric confidence interval, with $\alpha$ confidence level, from the following inequalities:

$$\underline{\mathrm{VMR}\,(X)} := \frac{\underline{\mathrm{Var}\,(X)}}{\widehat{\mathbb{E}\,(X)} + a_1} \leq \widehat{\mathrm{VMR}\,(X)} \leq \frac{\overline{\mathrm{Var}\,(X)}}{\widehat{\mathbb{E}\,(X)} - a_1} =: \overline{\mathrm{VMR}\,(X)}.$$

For a symmetric confidence interval with $\alpha$ confidence level (cf. Table 6), we simply take:

$$\widehat{\mathrm{VMR}\,(X)} \pm \max\left(\widehat{\mathrm{VMR}\,(X)} - \underline{\mathrm{VMR}\,(X)}, \overline{\mathrm{VMR}\,(X)} - \widehat{\mathrm{VMR}\,(X)}\right).$$

The $\mathcal{D}_2$ mean value for heat-shocks time gap $t_1 - (t_1 + \Delta t_1)$ is estimated using the confidence interval APMC method to verify the reward-based property:

$$\phi^i := \mathrm{R}_{\left\{\mathcal{D}_2^i=?\right\}}\left(\mathrm{I} = 1.05 \cdot (t_2 + \Delta t_2)\right)$$

where for $i = 1, 2$, first and second moment $\mathcal{D}_2$ rewards are defined as:

```
rewards
    "D_2^1" true: (S_2^max − S*)/(S_1^max − S*);
    "D_2^2" true: ((S_2^max − S*)/(S_1^max − S*))^2;
endrewards
```

Here, $\mathrm{S}_i^{\max}$ is an additional stochastic model variable, which is a witness of the maximum value of the substrate variable S, during and after the $i$-th heat-shock. Introduction of such variable in PRISM modelling language can be done seamlessly, i.e. without affecting the behaviour of the original CTMC. Finally, we have $\widehat{\mathbb{E}\,(\mathcal{D}_2)} = 1 - \phi^i$, as $\mathbb{E}\,(1 - X) = 1 - \mathbb{E}\,(X)$, and $\widehat{\mathrm{Var}\,(\mathcal{D}_2)} = \phi^2 - \left(\phi^1\right)^2$, as $\mathrm{Var}\,(1 - X) = \mathrm{Var}\,(X)$. The unbiased

standard deviation estimator $\widehat{\mathrm{SD}}\left(\mathcal{D}_2\right) = \sqrt{\widehat{\mathrm{Var}}\left(\mathcal{D}_2\right)}$, has the following $\alpha$ level confidence interval:

$$\sqrt{\underline{\mathrm{Var}\left(X\right)}} \leq \widehat{\mathrm{SD}}\left(X\right) \leq \sqrt{\overline{\mathrm{Var}\left(X\right)}},$$

provided that the variance estimator's precision is high enough, i.e. $\underline{\mathrm{Var}\left(X\right)} > 0$ (cf. Eq. (4)).

### S3.3: Approximate stochastic perturbation strategy

In our experiments we model scenarios of consecutive heat-shocks imposed on the model, separated with gaps. In principle, we control time points when the heat shocks are activated or inactivated. However, to do that in a probabilistic model one has to either save the whole distribution over a possibly infinite state space or, if analysis is based solely on stochastic simulations, modify the simulation algorithm to test again a current time point and queued deterministic events. Essentially, these are solutions based on moving to a more general type of models, like Markov decision processes, but the price to pay would be complication and impracticability of analysis (e.g., the APMC does not handle Markov decision processes).

We have thus chosen to consider heat-shock as an approximate random perturbation event and, thereby to stay within the same mathematical model and seamlessly perform stochastic simulations or model checking of CTMC.

Our approach relies on introduction of the sequence of $n_i$-counting Poisson processes (a special case of one-dimensional CTMC), independent of other state variables. Each time $i$-th process reaches value $n_i$, it is replaced by another $n_{i+1}$-counting Poisson processes with rate $n_{i+1} \cdot \tau_{i+1}$, where $1/\tau_{i+1} = t_{i+1} - (t_i + \Delta t_i)$, i.e. $\tau_{i+1}$ is an inverse of a time gap between perturbations $i$ and $i{+}1$. Because time between consecutive Poisson process events is exponentially distributed, i.e. $T_{ij} \sim \mathrm{Exp}\left(n_i \tau_i\right)$, the expected time for an approximate perturbation event equals to the time gap between deterministic perturbations time, i.e. $\mathbb{E}\left(\sum_{j=1}^{n_i} T_{ij}\right) = 1/\tau_i$. Moreover, due to independence of a time of occurrence of each count of the Poisson process $T_{ij}$, variance of the $i$-th perturbation event, calculated independently of prior $i-1$ perturbations, is equal to $\mathrm{Var}\left(\sum_{j=1}^{n_i} T_{ij}\right) = \sum_{j=1}^{n_i} \mathrm{Var}\left(T_{ij}\right) = 1/\left(n_i \tau_i^2\right)$. In other words the precision of a single $i$-th perturbation event, measured as a standard deviation, is proportional

by square root to the number of counting levels $n_i$ and inverse linearly proportional to the expected time of occurrence of this event $1/\tau_i$.

In PRISM modelling language we introduce two heat-shock events, i.e. four perturbation events of temperature parameter T, using Poisson processes with a common $n$ levels for each parameter and an additional perturbation number counter $i$. Using the compositional description of variables, which represent CTMC state, and *commands*, which change CTMC state, the independent perturbation events module (i.e. not synchronised with any other commands) is defined as:

```
ctmc
const double t1; // time offset for 1st heat-shock
const double td1; // duration of 1st heat-shock
const double t2; // time offset for second heat-shock
const double td2; // duration of 2nd heat-shock
const int Td; // heat-shock temperature delta
const int n; // event switcher levels

module events
    i : [0..4] init 0; // number of perturbation
    ps: [0..1] init 0; // perturbation switcher
    cnt: [1..n] init 1; // actual poisson process variable

    //pre 1st heat-shock
    [] i = 0 & cnt < n -> n/t1: (cnt'=cnt+1);
    [] i = 0 & cnt = n -> n/t1: (i'=1)&(ps'=1)&(cnt'=1);

    //1st heat-shock
    [] i = 1 & cnt < n -> n/td1: (cnt'=cnt+1);
    [] i = 1 & cnt = n -> n/td1: (i'=2)&(ps'=0)&(cnt'=1);

    //pre 2nd heat-shock
    [] i = 2 & cnt < n -> n/t2: (cnt'=cnt+1);
    [] i = 2 & cnt = n -> n/t2: (i'=3)&(ps'=1)&(cnt'=1);

    //2nd heat-shock
    [] i = 3 & cnt < n -> n/td2: (cnt'=cnt+1);
    [] i = 3 & cnt = n -> n/td2: (i'=4)&(ps'=0)&(cnt'=1);
endmodule

formula T = (37+Td*ps); // temperature for misfolding rate
```

Clearly, increasing $n$ increases number of states of the model, hereby making the experiments less efficient. A suitable value of parameter $n$ has been chosen experimentally by visual assessment of the precision of substrate stochastic trajectories, taking under consideration simulations efficiency; see caption in Figure 2 for details.

**Figure 2:** Comparison of simulations of approximate perturbations in the stochastic model with respect to RRE numerical solutions. The comparison is shown for different levels $n$ of the independent Poisson process, which approximates the deterministic scheme of perturbations of the temperature (left column). Plots show examples of 10 stochastic simulations, and mean $+/-$ standard deviation, estimated from 1000 samples, for the temperature perturbation scheme (left column) and the substrate amount (right column). Variance of time of a temperature perturbation event $T$ is a function of an perturbations time gap $t$ and the precision levels $n$, i.e. $\mathrm{Var}\,(T) = t^2/n$. Therefore, the main single time point approximation error for our perturbation scheme lies within an event of the second heat-shock with $t = 343\ \mathrm{min}$ (cf. left column). Note though, that errors for subsequent perturbation times accumulate, so the biggest error can be observed for the end of the second heat shock. Nevertheless, because start of the second heat-shock creates high amounts of molecules in the system, it is the most error influencing event, with respect to species amounts expected from RRE numerical solutions (cf. right column). We found that for $n = 2^{13}$ the approximation of mean and standard deviation of the substrate amount in the second heat-shock is in a good agreement with much more precise values in the first heat-shock and with RRE solutions.

**Figure on the next page.**

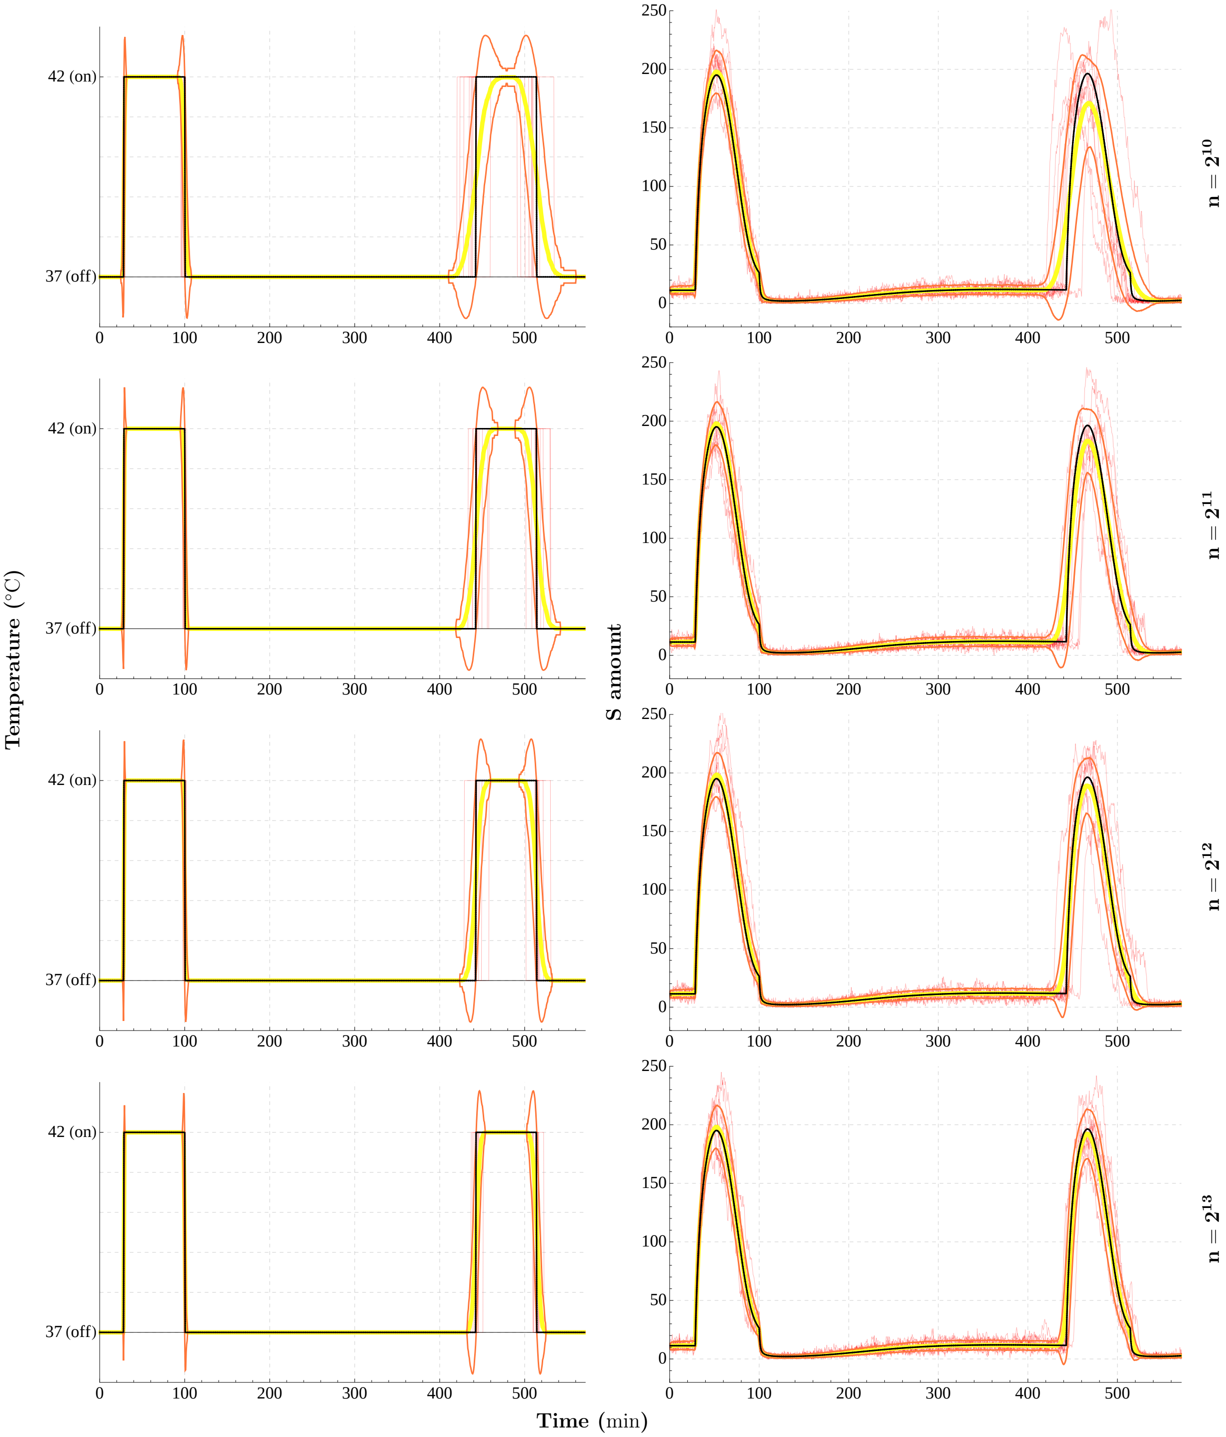
Temperature (°C)
42 (on)
37 (off)
S amount
Time (min)
n = $2^{10}$
n = $2^{11}$
n = $2^{12}$
n = $2^{13}$

# Supporting References


[1] Abravaya, K., Phillips, B., Morimoto, R.I.: Attenuation of the heat shock response in HeLa cells is mediated by the release of bound heat shock transcription factor and is modulated by changes in growth and in heat shock temperatures. Genes Dev 5(11), 2117–2127 (1991)

[2] Charzyńska, A., Nałecz, A., Rybiński, M., Gambin, A.: Sensitivity analysis of mathematical models of signaling pathways. BioTechnol 93(3), 291–308 (2012)

[3] Lepock, J.R., Frey, H.E., Ritchie, K.P.: Protein denaturation in intact hepatocytes and isolated cellular organelles during heat shock. J Cell Biol 122(6), 1267–1276 (1993)

[4] Milo, R., Jorgensen, P., Moran, U., Weber, G., Springer, M.: BioNumbers–the database of key numbers in molecular and cell biology. Nucleic Acids Res 38(Database issue), D750–753 (2010)

[5] Mizera, A., Gambin, B.: Stochastic modelling of the eukaryotic heat shock response. J Theor Biol 265(3), 455–466 (2010)

[6] Peper, A., Grimbergen, C.A., Spaan, J.A., Souren, J.E., van Wijk, R.: A mathematical model of the hsp70 regulation in the cell. Int J Hyperther 14(1), 97–124 (1998)

[7] Petre, I., Mizera, A., Hyder, C.L., Meinander, A., Mikhailov, A., Morimoto, R.I., Sistonen, L., Eriksson, J.E., Back, R.: A simple mass-action model for the eukaryotic heat shock response and its mathematical validation. Nat Comp 10(1), 595–612 (2011)

[8] Szymańska, Z., Żylicz, M.: Mathematical modeling of heat shock protein synthesis in response to temperature change. J Theor Biol 259(3), 562–569 (2009)

[9] Wilkinson, D.J.: Stochastic Modelling for Systems Biology. CRC Press (2011)
